# Supplementary material for: Sparsh: Self-supervised touch representations for vision-based tactile sensing
Source: arXiv:2410.24090 source file (2024-10-31)
Supplement: Supplementary file 1 [file arch_table.tex]

% \begin{table}[t]
% \centering
% \small
% \begin{tabular}{@{}l cccc}
% \toprule
% Arch.     & Loss   & Heads & Blocks & FFN layer    \\
% \midrule
% \mae        & 768           & 6    & 12     & MLP        \\ 
% \dino        & 768           & 12    & 18     & MLP        \\ 
% \ijepa       & 768          & 16    & 24     & MLP        \\ 
% \vjepa     & 788          & 16    & 24     & SwiGLU   \\ 
% \bottomrule
% \end{tabular}
% \caption{
% \textbf{Architecture details of the ViT-S/B/L/g networks used in this work.} \todo{Copied from DINOv2 please FIX!!} We use MLP feed-forward networks for distilled models, and SwiGLU ~\citep{shazeer2020glu} when training from scratch.
% }
% \label{tab:vit-hparams}
% \end{table}

% SSL METHODS
\begin{table}[!t]
% \GobbleLarge
\centering
\small
\begin{tabular}{@{}ccccc@{}}
\toprule
Model &
  Input &
  \begin{tabular}[c]{@{}c@{}}SSL\\ Framework\end{tabular} &
  \begin{tabular}[c]{@{}c@{}}Data\\ Augmentation\end{tabular} &
  \begin{tabular}[c]{@{}c@{}}Loss\\ Function\end{tabular} \\ \midrule
  \mae &
  \multirow{3}{*}{2 images $(h \times w \times 6)$} &
  Generative &
  Random Masking &
  \begin{tabular}[c]{@{}c@{}}$\Lv_2$ \\ pixel space\end{tabular} \\ [0.2cm]
  
  \dino &
   &
  Distillation &
  Block Masking &
  Cross-Entropy \\ [0.1cm]
  
  \ijepa &
   &
  \multirow{2}{*}{\begin{tabular}[c]{@{}c@{}}Joint-\\Embedding\\ Predictive\end{tabular}} &
  Multi-Block Masking &
  \begin{tabular}[c]{@{}c@{}}$\Lv_2$\\ latent space\end{tabular} \\ [0.1cm]
  \vjepa &
  4 images $(t \times h \times w \times 3)$ &
   &
  % \begin{tabular}[c]{@{}c@{}}Random Tube\\ Masking\end{tabular} &
  Random Tube Masking &
  \begin{tabular}[c]{@{}c@{}}$\Lv_1$\\ latent space\end{tabular} \\ \bottomrule
\end{tabular}
\caption{\textbf{Exploration of SSL Frameworks for Tactile Representation Learning.} We applied four SSL methods to determine the most suitable approach for learning representations in the domain of vision-based tactile images. All models use as encoder a ViT-B architecture, where the embedding dimension is 784.}
\label{tab:ssl_methods_comparison}
\normalsize
% \GobbleLarge
\end{table}
